# Supplementary material for: In-Context Learning with Noisy Labels
Source: arXiv:2411.19581 source file (2024-11-29)
Supplement: Supplementary file 1 [file A_appendix.tex]

\clearpage
\section{Appendix}\label{sec:6_appendix}
\noindent\textbf{Dataset Details.}
In this section, we show our dataset configuration details.
Following the previous work~\cite{ye2023compositional}, the training dataset has split into $90 : 10$ train / validation set and the final scores are measured on the original validation set.
Our 3 datasets are described as below:

\begin{table}[]
\begin{tabular}{@{}llll@{}}
\toprule
Dataset & \# train data & \# validation data & Formatting                                                                                                      \\ \midrule
MRPC    & 3,668         & 408                & \textbackslash{}texttt\{\{sentence1\} Can we say \textbackslash{}"\{sentence2\}\textbackslash{}"? \{Yes, No\}\} \\
SST-5   & 8,534         & 1,101              & \textbackslash{}texttt\{\{sentence\} It is \{terrible,bad,OK,good,great\}\}                                     \\
Tweet   & 9,000         & 1,000              & \textbackslash{}texttt\{Tweet: \{sentence\} \textbackslash{}n Hate: \{Yes, No\}\}                               \\ \bottomrule
\end{tabular}
\label{tab:data_config}
\end{table}
\begin{itemize}
    \item \textbf{MRPC \cite{dolan2005mrpc}} is a dataset for paraphrase detection task, where each data consists of a pair of sentences collected from online newswire articles and a label indicating whether it is a paraphrase or not. 
    %The label space is the set $\{\texttt{yes,no}\}$ and it has $3,668$ training and $408$ validation examples.
    \item \textbf{SST-5 \cite{socher2013sst5}} consists of single sentence examples extracted from movie reviews. Each of example is labeled in 5 classes ranging from "very negative" to "very positive". Note that we converted the label space as $\{\texttt{terrible,bad,OK,good,great}\}$ to map the labels to single words~\cite{ye2023compositional}. 
    %It has $8,534$ and $1,101$ training / validation examples.
    \item \textbf{Tweet hate speech detection(\cite{basile-etal-2019-semeval}}) consists of english tweet data. Each sample contains a hate speech about women or immigrants or not.
\end{itemize}

We summarize dataset information and our formatting template in Table \ref{tab:data_config}

\noindent\textbf{Training Details.}
To train a BERT classification model, we fine-tune it for 30 epochs with batch size of 64 and learning rate of 5e-5.
For the rectifying network, we fine-tune it for for 10 epochs with batch size of 2 and learning rate of 1e-4, employing LoRA~\cite{hu2022lora} for memory-efficient training.
Lastly, for the GPT-2 classification model in Section \ref{subsec:4_3_results_analysis}, we fine-tune the same base model with the rectifying network (without changing the last layer as the classifier head). We trained it for 8 epochs, batch size of 16, and learning rate of 1e-4.
All of our experiments are conducted on two NVIDIA A5000 GPUs, and we utilize FSDP~\cite{Zhao2023fsdp} to avoid the memory limitation.
